# Supplementary material for: SGDRC: Software-Defined Dynamic Resource Control for Concurrent DNN Inference on NVIDIA GPUs
Source: arXiv:2407.13996 source file (2025-03-26)
Supplement: Supplementary file 1 [file text.tex]

After briefly introducing the architecture of \textsc{Missile}, we now demonstrate how \textsc{Missile} eliminates intra-SM resource contention based on \textit{elastic spatial-temporal SM multiplexing}.

\PHM{SM spatial isolation.} \textsc{Missile} used \texttt{libsmctrl}~\cite{Bakita2023}, a library that manipulates Task Meta Data (TMD, an NVIDIA's little-known data structure~\cite{tmd-patent}), to control the set of TPCs to which each launched kernel can be assigned. This library is compatible with all commercially available NVIDIA GPUs and the latest CUDA version.

%\begin{figure}
%	\centering
%	\includegraphics[width=\columnwidth]{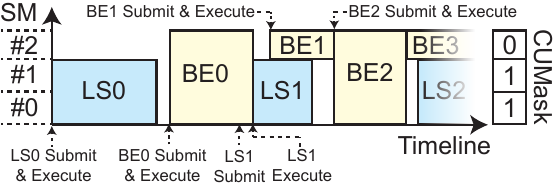}
%	\caption{Illustration of \textsc{Missile}'s SM placing scheme. An LS task and a BE task run concurrently on a GPU with three TPCs, with their kernels being named with prefixes \texttt{LS} and \texttt{BE}, respectively.}
%	\label{fig:sm_masking}
%\end{figure}

\PHM{SM temporal isolation.} Now, we assign dedicated SM units to LS and BE tasks separately. To enhance the utilization of SM units, we allow different LS and BE tasks to share their respective SM units in a time-multiplexed manner. %Given that the kernel runtime for LS services is typically extremely short (usually ranging from \revised{0.001} ms to 0.05 ms), we synchronize \revised{LS kernel launch stream} in batches when dispatching DNN kernels in a time-multiplexed manner to minimize the overhead of stream synchronization after launching the kernels. \revised{During each round of kernel launch, we sequentially select kernels from the LS kernel queues and accumulate their runtimes $R_i$ (obtained through offline profiling) until $\sum R_i$ exceeds the threshold $T_R$. Then, we launch these kernels in a group and wait for synchronization. By analyzing the overhead of \texttt{cuStreamSynchronize}, we set $T_R$ = ?? ms.}

\PHM{Elastic \revised{SM multiplexing}.} \textsc{Missile} elastically auto-scales batch tasks' SM allocation to maximize the SM utilization. During the execution of LS kernels, BE kernels exclusively utilize the SMs that are not occupied by LS tasks. For example, if LS services occupy 70\% of the SMs, BE kernels will allocate and utilize only the remaining 30\% of the SMs. In the absence of any running LS kernel, BE tasks will aggressively occupy all available SMs. However, this approach introduces a challenge: when an LS kernel arrives, all SMs might be occupied by BE tasks, posing difficulty in swiftly scheduling the LS kernel onto the GPU. To address this, we implemented fast BE kernel preemption by transforming BE kernels, which follows FLEP's design~\cite{Wu2017}. An illustrative example of BE kernel transformation is presented in Fig.~\ref{fig:dnn_kernel_transformation_example}.

%\subsection{Batch Task Preemption}
